# Supplementary material for: Run-Based Semantics for RPQs
Source: arXiv:2211.13313 source file (2022-11-23)
Supplement: Supplementary file 1 [file iterative-simple.tex]

\newappendix{Emptyness is untractable under iterative-simple run semantics (deprecated)}

We reuse the definition from the main text. In particular, our model for graph databases is defined is \rsection{data-mode}, RPQs in \rsection{quer}, and computational problems in~\rsection{comp-prob}

\begin{proposition}\lproposition{itera}
    With the RPQ~$R=(a^*ba^*)^*$, problem \problemfont{Tuple membership} is NP-hard under iterative-simple run semantics.
\end{proposition}
\begin{proof}
    Reduction is done to \problemfont{Two disjoint path} \cite{something}
    and the proof is similar.
    Indeed, the input of \problemfont{Two disjoint path} is a graph~$G$ and two node pairs~$(s_1,t_1)$ $(s_2,t_2)$, and without loss of generality we assume that all elements in~$\set{s_1,t_1,s_2,t_2}$ are pair-wise distinct.
    We construct a database~$D$ as follows: copy~$G$, label all edges with letter~$a$, add one fresh node~$M$ and two fresh edges~$t_1\rarrow{b} M$
    and~$\rarrow{s_2}$.
    
    Consider a walk~$w$ in~$D$ that matches~$R$ under iterative-simple run semantics.  Since the elements in~$\set{s_1,t_1,s_2,t_2}$ are pair-wise distinct, the length of~$w$ is not zero. 
    Thus~$w$ passes by~$M$ since the only the only labelled by~$b$.
    Since~$M$ has exactly one incoming and one outgoing edge,~$w$ has to use both. 
    Since~$w$ satisfy iterative-simple run semantics,~$w$ use these two edges exactly once each, hence~$w$ may be decomposed as
    \begin{equation}
        w=\underbrace{s_1 \rarrow{}\cdots\rarrow{}t_1}_{\overflow{r}{w_1={}}}
        \rarrow{b} M \rarrow{b}
        \underbrace{s_2 \rarrow{}\cdots\rarrow{}t_2}_{\overflow{r}{w_2={}}}\quad,
    \end{equation}
    where the labels in~$w_1$ and~$w_2$ are both in~$a^*$.
    The walk~$w_1$ (resp.~$w_2$) is matched by the first (resp.~second) occurrence of~$a^*$, hence due to iterative-simple run semantics,~$w_1$ (resp~$w_2$) is a simple walk.
    Since~$w_1$ and~$w_2$ are matched by the same sub-expression under a star, they are disjoint.
\end{proof}

%\begin{remark}
%    The class of RPQs for which \problemfont{Tuple Membership} is NP-Hard under iterative-simple run semantics is not clear.
%    For instance, the reduction above would not work with a query such as~$(a^*b)^*$ (although it would for instance with simple walk or trail semantics).  Indeed in that case, simple-run semantics and iterative-simple run semantics coincide.
%\end{remark}

It is also untractable for some expressions of star-height 1.

\begin{proposition}
    With RPQ~$(baa)^*$, problem \problemfont{Tuple membership} is NP-hard
    under iterative-simple run semantics.
\end{proposition}
\begin{proof} Once again, the reduction is done from \problemfont{Two Disjoint walk}, but this time the database has to be constructed.

Let~$G$ be the graph, and~$(s_1,t_1)$ $(s_2,t_2)$ be the two nodes pairs
that are given as input to \problemfont{Two Disjoint Path}.
Without loss of generality we assume that all elements in~$\set{s_1,t_1,s_2,t_2}$ are pair-wise distinct.
We construct a database~$D$ from~$G$ as follows. 
\begin{itemize}
    \item Copy all nodes from~$G$ into~$D$.
    \item For every edge~$(s,t)$ of~$F$ we add a copy of the following gadget to~$D$.
    
    \begin{figure}[h!]\centering
    \begin{tikzpicture}
        \node[node] (s) {$s$};
        \path (s)  ++(0:\nodedist) node[node] (a) {} 
                   ++(30:\nodedist) node[node] (aa) {} 
                   ++(-30:\nodedist) node[node] (t) {$t$};
        \path (a)  ++(-30:\nodedist) node[node] (ab) {};
        \path[edge] (s) to node[above] {$a$} (a);
        \path[edge] (a) to node[above left] {$a$} (aa);
        \path[edge] (a) to node[below left] {$b$} (ab);
        \path[edge] (aa) to node[above right] {$b$} (t);
        \path[edge] (ab) to node[below right] {$a$} (t);
    \end{tikzpicture}
    \caption{Gadget to insert in~$D$ for each edge~$(s,t)$ in $G$}
    \end{figure}

    \item Add two fresh nodes $start$ and $end$
    \item Add three edges: $start\rarrow{b}s_1$, $t_1\rarrow{a}s_2$ and $s_1\rarrow{a}end$; we call those the \emph{special edges}.
\end{itemize}
We instantiate \problemfont{Tuple membership} with database~$D$, RPQ $(baa)^* $ and tuple~$(Star,End)$, and claim that it is equivalent to \problemfont{two disjoint paths}.

Note that any word matching~$(b(aab)^*a(aba)^*a)$ also matches~$(baa)^*$. 
Inver

Let~$w$ be any walk in~$D$ matching~$(baa)^*$ and that foes from $start$ to $end$.
It has a length divisible by three, and necessarily uses two special edges, hence it necessarily uses the third one.
As a result,~$w$ may be decomposed as:
\begin{equation}
    start \rarrow{b} 
    \underbrace{s_1 \rarrow{u_1} t_1}_{\overflow{r}{w_1=}}
    \rarrow{a}
    \underbrace{s_2 \rarrow{u_2} t_1}_{\overflow{r}{w_2=}}
    \rarrow{a} end
\end{equation}
where~$u_1$ matches~$(aab)^*$ and~$u_2$ matches~$(aba)^*$,
and where the three other edges above are the three special edges.
It is quite easy to see that by construction, three consecutive nodes in~$w$ are always pair-wise distinct.  Hence, iterative-simple semantics ensures that~$w_1$ is a simple walk.

\end{proof}
