# Supplementary material for: Run-Based Semantics for RPQs
Source: arXiv:2211.13313 source file (2022-11-23)
Supplement: Supplementary file 2 [file AG-example.tex]

\newappendix{Example from \cite{RobinsonWebberEifrem2015} that fails due to trail semantics}
