# Supplementary material for: Run-Based Semantics for RPQs
Source: arXiv:2211.13313 source file (2022-11-23)
Supplement: Supplementary file 3 [file cypher-like-query.tex]

\newappendix{Cypher-like query}
\label{a:cyph-like}
