# Supplementary material for: Run-Based Semantics for RPQs
Source: arXiv:2211.13313 source file (2022-11-23)
Supplement: Supplementary file 5 [file old_intro.tex]

\newappendix{Old introduction}

\section{Introduction}

The formalism of Regular Path Queries (RPQs) is one of the main building blocks of most languages for querying graph databases.
%
It is highly studied in the literature \cite{things}



\paragraph{Computation problems}
For references, we give here a brief descriptions of some computational problems of interest.  We consider a graph database as input, and an RPQ~$R$ as parameter.
The problem of deciding if there exists no walk matching $R$ is called  \problemfont{Emptiness}.
the problem \problemfont{Tuple membership} is similar but we are interested only in the walks that span between two endpoints given as extra input; it is computationally equivalent to \problemfont{Emptiness}.
%
We call \problemfont{Walk enumeration} the problem of enumerating all the walks that match the query.
The problem of \problemfont{Walk counting} consists in outputting the number of walks matching the query.
The precise semantics used is also a parameter of the problem and should be clear from context.


Note that \problemfont{Walk enumeration} and \problemfont{Walk counting} have no meaning under walk semantics since the result may be infinite.  On the other hand \problemfont{Emptiness} and \problemfont{Tuple membership} can be solved very efficiently \cite{something}.
On the other hand, most graph-database management systems decided not to use the classical walk semantics, and it seems it is precisely because they
want to treat walks as first class citizens, and in particular because the users want to be able to enumerate and count matching walks. 
We list below a few of the approaches for adapting walk semantics.

\paragraph{Topological restriction}  This approach is based on filtering out some of the matched walks when they contain some ``redundancy": e.g., repeated edges are forbidden in trail semantics, or repeated nodes are forbidden in simple walk semantics.
In particular, topological restrictions are such that only a finite number of walks are kept.

For instance, \emph{trail semantics} is known for being implemented in the famous language Cypher \cite{FrancisEtAl2018,FrancisEtAl2018-arxiv}.
The language GQL\cite{DeutschEtAl2021} features several topological restrictions: with the keyword \gqlinline|TRAIL| only trails are returned, with the keyword \gqlinline|SIMPLE| only simple cycles or walks are returned, and with the keyword \gqlinline|ACYCLIC| only simple walks are returned.

The main issue with this approach is that most computational problems become untractable even for some fixed queries.
For instance, there are RPQs such that deciding \problemfont{Emptiness} is NP-complete in the size of the database.  It is already the case for some simple RPQs such as $a^*ba^*$ or $(aba)^*$; see \cite{MartensNiewerthTrautner2020} for trail semantics and \cite{BaganBonifatiGroz2020} for simple-walk semantics.
As a result, most other computational problems, such as \problemfont{Walk enumeration} or \problemfont{Tuple Multiplicity}, are also untractable in data complexity.

Another issue comes from the fact that the topological restriction chosen is arbitrary, in the sense that it is globally imposed to the user.  
Hence, it is prone to error.
Let us give an anecdotal example about trail semantics and Cypher.
The introductory book \emph{Graph databases} \cite{RobinsonWebberEifrem2015} contains
a chapter that presents \emph{real-world examples} and there is one use-case about \emph{Geospatial and Logistics}, starting on page 132; the actual query is given in page 139.
We cannot reproduce the full example here, since it takes several pages to be written and explained.
It boils down to the following. The database is a DAG\footnote{DAG stands for Directed Acyclic Graph} with a root (that is, a vertex that may reach all other vertices), and one wants to write a query to find the best route to go from one specific leaf back to the root and then forward to another specific leaf.
(It is explicitly said that the route must pass though the root due to logistic reasons.)
One may see that in that scenario the best route might use twice the same edge, something that is forbidden by trail semantics.
Hence, the query must be written with particular care in order to circumvent trail semantics, and it was not the case in the example, probably because the complicated part of the query is supposed to be elsewhere.
%It is possible to circumvent trail semantics and write a correct query, but it requires a fine understanding of the semantics, which users usually do not have.
% Note that this query is particularly nasty for the following reasons.
% First, aggregation is used after pattern matching, hence it is hard to adapt the query in order to circumvent trail semantics. % VM: this is false
% Second, the query computes a "best route" for some metrics, hence the mistake is unlikely to be spotted by tests.
% Third, even without topological restrictions, the query would have a finite number of matches; this fact probably explains why the author of the query did not think about trail semantics.
%One may modify the query to circumvent the topological restriction, but 







\paragraph{Reduction of expressive power}
In the absence of topological restriction or endpoint-based selection, the language GQL will simply forbid the use of a Kleene star altogether.
Note that with that restriction, Conjunctions of RPQs (CRPQs) are of the same expressive power as conjunctive queries (CQs).
    
\paragraph{Changing the semantics depending of the fragment used}
The language SPARQL\footnote{SPARQL stands for SPARQL Protocol and RDF Query Language} initially allowed only CQs, and used walk semantics with multiplicity. Note that in the case of CQs, there is only a finite number of matching walks.
Later on, SPARQL 1.1 introduced \emph{property paths} \cite{SPARQL1.1PP}, which allow the full extent of CRPQs, and finally decided to use walk semantics \textbf{without multiplicity}\footnote{It is an \emph{existential} semantics, in the sense that it does not allow to talk about the matched walk. Only \problemfont{Tuple Membership} has a meaning.}.
Since CRPQs contain CQs, applying this naively would mean that the result of CQs is different depending of whether it uses property paths.
It was decided that the semantics of property paths would compute multiplicity only if it was equivalent or a CQ, that in the absence of a Kleene star.

% deprecated
%Note that a different semantics has been suggested for the introduction of property paths in SPARQL 1.1; we call it \emph{iterative-simple run} semantics, and mention it because it bears some similarity with the semantics we propose here.
%In essence, iterative-simple run semantics filter out walks containing two subwalks that are matched by the same Kleene star and that have a vertex in common.
%In \cite{ArenasConcaPerez2012}, it was shown that \problemfont{Walk counting} 
%matching an expression as simple as $a^*$ is \#P-hard in the size of the database.
%We actually don't think this is as big a problem as they say, \rsection{s:tupl-mult}.
%On the other hand, it is quite easy to show using the techniques from \cite{MartensNiewerthTrautner2020} that under \emph{iterative-simple semantics}, 
%even \problemfont{Emptiness} is NP-hard for a fixed RPQ, typically $(a^*b)^*$ or $(aba)^*$.


\paragraph{Witness selection} 
This type of semantics comes from the fact that in problems such as
tuple membership, one often wants to get a witness of the membership,
in order to do further computation.
The typical is \emph{all-shortest-walk} semantics which gives as witnesses the shortest walks (the plural comes from ties).
It is the semantics in GSQL \cite{GSQL,DeutschEtAl2019}, and also will be available in GQL with keyword \gqlinline!ALL SHORTEST!.
Similarly, GQL allows \emph{any-shortest-walk} semantics, which non-deterministically choose exactly one of the shortest walks,
and \emph{any walk} which non-deterministically choose one arbitrary walk.

For problems where endpoints are not given as input, such as \problemfont{Walk enumeration}, matching walks are partitioned by endpoint: each pair~$(s,t)$ of vertices defines a cell, which contains all matching walks going from~$s$ to~$t$.
Then, witness selection is applied independently on each cell.

This kind of semantics technically gives a meaning to \problemfont{Tuple multiplicity} but the intent is more to keep the output deterministic than
to enable multiplicities.
Indeed, it has a very different meaning than in other semantics.


\paragraph{Our proposal: run-based semantics}
In this article, we propose three semantics based on the same idea: \emph{simple run}, \emph{trail-run} and \emph{binding trail}.
 In order to keep the output finite, simple-walk semantics filter out the results that are considered to be redundant, that is, walks that use the same node twice. 
Our approach uses a finer notion of redundancy: redundancy in the matched walk is only forbidden when it coincides with redundancy in the computation of the query. For instance, under simple-run semantics, a matched walk is discarded only if it reuses a node and if the query computation did not progress compared to the previous times the node was seen.
Consider again the RPQ~$a^* b a^*$. For every semantics based on topological restriction, the untractability comes from the fact that the edges matched by the first occurrence of~$a^*$ cannot be.
It is similar in more complex cases, such as the RPQ~$(aba)^*$: the untractability also comes from the fact that an edge~$a$ that matches the first occurrence of $a$ forbids $e$ to match the second occurrence of $a$ later on.

Simple-run is defined on query that are given as automata.
Given the automaton-query~$\Ac$ and the database~$D$, we define the \emph{run-annotated database}, which is similar to the product~$\Ac\times D$, and call \emph{run} the walks in that structure.
A simple-run is thus a run that has no repeating vertex, and it is accepting if
its projection on its first component is an accepting computation of~$\Ac$.

\begin{theorem}
    \problemfont{Tuple Membership} under simple-run semantics coincide
    with \problemfont{Tuple Membership} under shortest-walk semantics.
\end{theorem}

\begin{corollary}
    \problemfont{Tuple Membership} is P-Time under simple-run semantics.
\end{corollary}

Similarly, since the structure is so simple, we may muster classical algorithms to answer most problems efficiently. In particular, using Yen Algorithm \cite{Yen71} (see also \cite{MartensNiewerthTrautner2020}) yields the following. 

\begin{theorem}
    \problemfont{Walk enumeration} is poly-delay under simple-run semantics.
\end{theorem}

However, it is quite easy to see that \problemfont{Tuple Multiplicity}
is \#P-Hard under simple-run semantics with a query as simple as~$a^*$.
This was seen as a deal-breaker in \cite{ArenasConcaPerez2012}, as the title suggests, but we disagree with their conclusion, or at least we do not think it applies to the property graph ecosystem.
Indeed, it is quite clear that no semantics will make \problemfont{Tuple Multiplicity} tractable, and thus the question is 
\emph{would you rather have counting impossible because it is undefined, or to have it being long to compute on hard instances?}
Past shows that in the property graph world, expressive power was often chosen over theoretical tractability. 
Hence, simple-run semantics seems to be a valid alternative to semantics used in real database engine.


\medskip

After preliminaries, where we present in particular our data model, we define 
our run-based semantics framework in \rsection{run-base}.
Then, \rsection{comp-prob} defines the computational problems and give their complexity; in addition to those presented in this introduction, we also show that \problemfont{Walk membership} is NP-Hard in data complexity for simple-run semantics.

\paragraph{Queries as expressions}
In real-life, queries are given as regular expression, and not as automaton, and since simple-run semantics changes depending on the automaton, the choice of the expression-to-automaton algorithm is crucial.  We briefly discuss  this topic in \rsection{quer-as-expr} and conclude that the Glushkov construction seems to
be the best solution. We then show that one cannot hope to muster the special form of the Glushkov automaton to obtain better upper-bounds.  Indeed, we show a very general statement stating that one can devise an expression~$R_\Ac$ in such a way that the Glushkov automaton built from~$R_\Ac$ encodes the behavior and topology of an arbitrary automaton~$\Ac$ (\rdefinition{topo-codi} and \rtheorem{topo-codi-glus}).
